# Supplementary material for: StyleVideoGAN: A Temporal Generative Model using a Pretrained StyleGAN
Source: arXiv:2107.07224 source file (2021-11-30)
Supplement: Supplementary file 1 [file supplemental_arxiv.tex]

\documentclass{bmvc2k}

\include{includes}

\include{commands}

\toggletrue{arxiv}

\input{core_supplemental}
